# Supplementary material for: Width-dependent Photoluminescence and Anisotropic Raman Spectroscopy from Monolayer MoS$_2$ Nanoribbons
Source: arXiv:1709.04001 ancillary file (2017-09-12)
Supplement: Supplementary file 1 [file Wei_2017_SupplementaryInformation.pdf]

# Supplementary Material for: Width-dependent Photoluminescence and Anisotropic Raman Spectroscopy from Monolayer $MoS_2$ Nanoribbons

Guohua Wei[1], Erik J. Lenferink[2], David A. Czaplewski[3], and Nathaniel P. Stern[2]

[1]*Applied Physics Program, Northwestern University, Evanston, IL 60208, USA*
[2]*Department of Physics and Astronomy, Northwestern University, Evanston, IL 60208, USA*
[3]*Center for Nanoscale Materials, Argonne National Laboratory, Argonne, IL 60439, USA*

September 11, 2017

## 1 Fabrication of monolayer $MoS_2$ nanoribbons

A typical process for creating nanoribbon structures with electron beam (e-beam) lithography involves directly exposing ribbon arrays using a negative resist with extremely high doses. Although this is suitable for conducting graphene [1], the e-beam can cause damage in semiconductor materials such as monolayer $MoS_2$. The high-resolution e-beam lithography system we use operates at 100 kV. Since direct exposure of monolayer $MoS_2$ to an electron beam degrades the material's optical quality and electrons with energy greater than 80 keV can break Mo-S bonds and introduce structural defects [2, 3], patterning methods requiring high dose e-beam exposure are not acceptable [4]. Instead of the typical negative resist, we use a positive resist and write channels on the two sides of a ribbon with high-resolution e-beam, as shown in Fig. S1.

The exfoliated monolayer flake is coated with a positive resist (GL2000) with a thickness over 40 nm. After e-beam exposure and cold development (-5℃), the resist nanowire array is transferred onto the flake. During this step, the resist wires are typically about 40 nm wide, with some size control obtained using dose modulation. A reactive ion etch (RIE) is performed following the e-beam patterning process. The RIE conditions are 20/10 sccm for

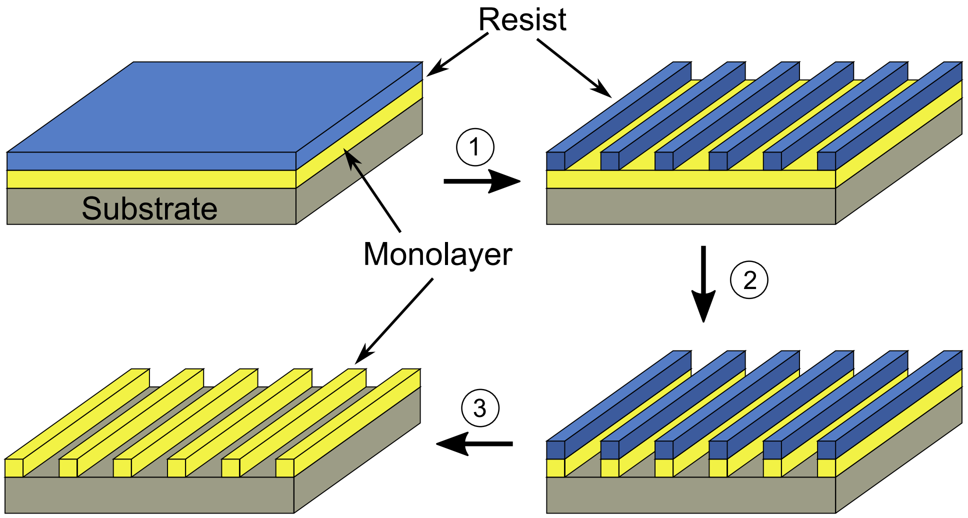


**Figure S1:** Illustration of the fabrication process for monolayer $MoS_2$ nanoribbons. Step 1 indicates exposure and development of the resist (blue). Step 2 shows the RIE etching process removing the exposed monolayer (yellow). Step 3 is the resist removal to reveal the patterned ribbons underneath.

$CHF_3/O_2$ gas flow with 30 W RF power at a pressure of 50 mTorr. The etching time is $20 - 50$ seconds depending on the desired size.

To quantify ribbon width, AFM scans are taken. Two representative ribbon arrays are shown in Fig. S2. There is some resist residue after the removal process. Since the resist residue is only a couple nanometers thick, it is thin enough to extract the ribbon width with reasonable accuracy. A fit of the height profile to a Gaussian function quantifies the ribbon width. Carefully controlling the etch conditions can create wires with variable widths around 20 nm.

## 2 Fitting Polarization Resolved Raman Intensities

In polarized Raman spectroscopy, the intensity of scattered light is measured as a function of its polarization angle to incident. The intensities of scattered Raman modes are determined by the Raman tensors, which can be expressed as $I = |\boldsymbol{e_s^t} \cdot R \cdot \boldsymbol{e_i}|^2$ [5, 6], where $\boldsymbol{e_i}$ and $\boldsymbol{e_s}$ are the unit vectors for the incident and scattered light electric fields, the superscript $t$ is the transpose of the column vector to a row vector, and $R$ is the Raman tensor determined by the crystal symmetry. Polarized Raman spectroscopy is thus a useful technique for studying crystal structural properties. Monolayer $MoS_2$ has two active Raman modes, $E'$ and $A'_1$, as

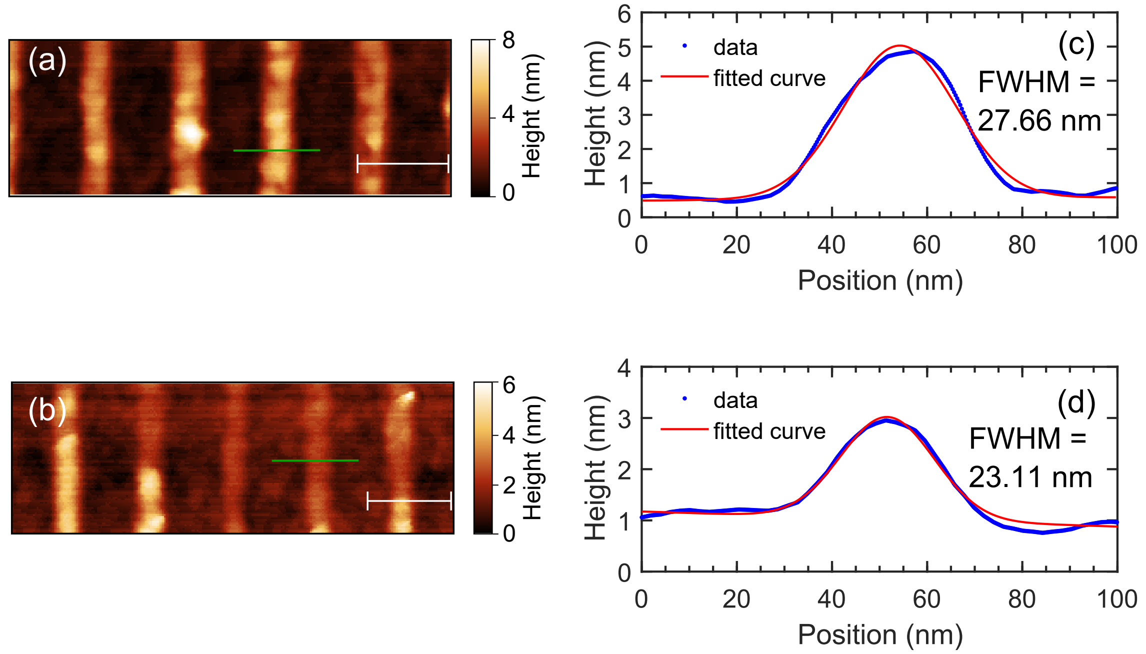


**Figure S2:** AFM of monolayer $MoS_2$ nanoribbons. (a-b) show the AFM images for ribbons with different sizes. The scale bars are 100 nm. (c-d) show the AFM height profiles along the green lines for (a) and (b) respectively, fit with Gaussian functions.

a result of its $D_{3h}$ crystal symmetry, which have corresponding Raman tensors: [5, 6]

$$R(A_1') = \begin{pmatrix} a & 0 & 0 \\ 0 & a & 0 \\ 0 & 0 & b \end{pmatrix}; \tag{S1}$$

$$R(E', (xy)) = \begin{pmatrix} 0 & c & 0 \\ c & 0 & 0 \\ 0 & 0 & 0 \end{pmatrix}; R(E', (x^2 - y^2)) = \begin{pmatrix} d & 0 & 0 \\ 0 & -d & 0 \\ 0 & 0 & 0 \end{pmatrix} \tag{S2}$$

where the in-plane mode $E'$ has two active components for cross polarization (incident light perpendicular to scattering light) $R(E', (xy))$, and parallel polarization $R(E', (x^2 - y^2))$. Choosing the monolayer to be in the $x - y$ plane, the incident light electric field can be written as $\boldsymbol{e_i} = (\cos\theta, \sin\theta, 0)$ when its polarization angle is $\theta$ to the $x$ direction (Fig. 1(b) in main text). In the back scattering geometry, when the collection analyzer is polarized along the X axis, the scattered light polarization after the analyzer can be written as $\boldsymbol{e_s} = (1, 0, 0)$. The corresponding Raman intensity is $I(A_1') = |\boldsymbol{e_s^t} \cdot R(A_1') \cdot \boldsymbol{e_i}|^2 = a^2 \cos^2\theta$ for $A_1'$ mode. Likewise, $I(E') = d^2 \cos^2\theta + c^2 \sin^2\theta$ for $E'$ mode. Since $d \approx c$, the $E'$ mode is almost angle independent while the $A_1'$ mode is polarization-dependent in monolayer $MoS_2$.

The Raman mode scattered by $R(E')$ has two polarized components, where $\boldsymbol{R}(xy)\boldsymbol{e_i} = c(\sin\theta, \cos\theta, 0)$ is perpendicular to the excitation laser, and $\boldsymbol{R}(x^2-y^2)\boldsymbol{e_i} = d(\cos\theta, -\sin\theta, 0)$ is parallel to the excitation laser. The measured intensity follows $\eta(\theta)d^2+\eta(\theta-90°)c^2$, where $\eta(\theta) = 0.52+0.48\cos^2(\theta+5°)$ is the angle-dependent detection efficiency, derived by detector calibration. The fit to this equation of the monolayer Raman modes measured *without* the analyzer (Fig. 2(a)) gives $c/d = 0.79 \pm 0.05$. The Raman spectra measured *with* the analyzer (Fig. 1(d)) gives a similar $c/d$ ratio ($c/d = 0.84 \pm 0.01$), which confirms the analysis here. (In this case $c/d = \sqrt{I_{90°}/I_{0°}}$.)

The same measurements are carried out for the nanoribbons. Figure 1(e) and Fig. 2(b, c) show the polarization anisotropy for nanoribbons measured with and without analyzer, respectively. Fitting the $I(E')$ measured *with* analyzer using the equation $I(E') = d^2\cos^2\theta + c^2\sin^2\theta$ gives $c/d = 0.67 \pm 0.02$. However the $I(E')$ measured *without* analyzer could not be fit with the assumption that the tensor parameters are independent of incident polarization, in other words, the Raman tensors are anisotropic.

# 3 Size effects on Raman spectra

In a first-order Raman scattering process, energy and momentum conservations only permit optical phonons near the Brillouin zone center to interact with incident photons ($\boldsymbol{q} \approx 0$). However, this requirement is relaxed in a finite system where the uncertainty principle allows phonons with momentum in the range of $|\boldsymbol{q}| < 1/W$ to be involved in the process, where $W$ is the ribbon width.

For single phonon scattering, the Raman intensity follows [7, 8]

$$I(\omega) \propto \frac{1}{(\omega-\omega_0)^2 + (1/2\Gamma)^2} \tag{S3}$$

where $\omega_0$ is the Raman shift frequency (phonon frequency), $\Gamma$ is the corresponding linewidth broadening. Considering a Gaussian phonon wavepacket, in the nanoribbon case

$$I(\omega) \propto \int \frac{\exp(-\boldsymbol{q}^2W^2/16\pi^2)}{(\omega-\omega(\boldsymbol{q}))^2 + (1/2\Gamma)^2}\,\mathrm{d}\boldsymbol{q} \tag{S4}$$

For the first order approximation, one can consider a one-dimensional phonon dispersion and assume that the scattering cross-section is identical for all phonons. Following the calculations in Ref. [9], the $E'$ mode dispersion can be written as $\omega_E(q) = 385 - 10\sin(qa)$ cm$^{-1}$,

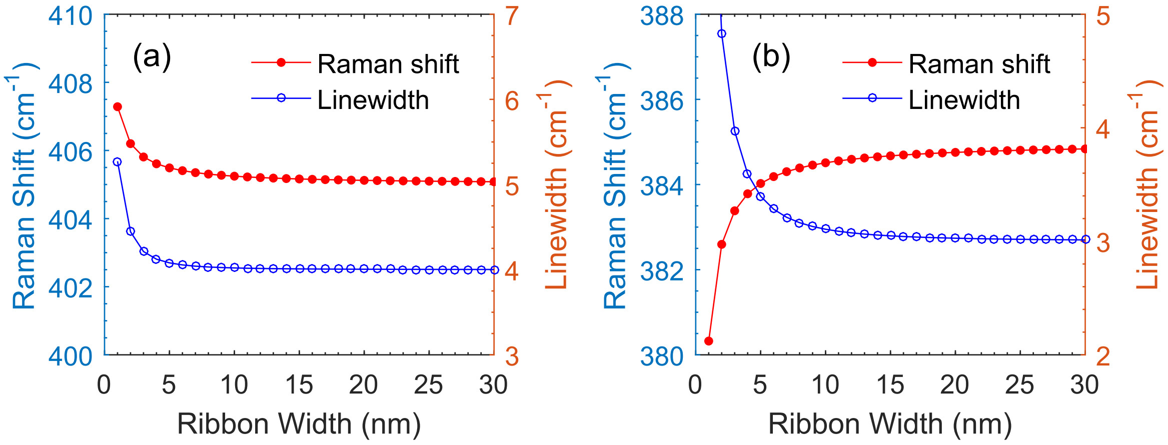


**Figure S3:** Calculated size-dependent Raman shift and linewidth of monolayer $MoS_2$ nanoribbons for the $A_1'$ mode (a) and the $E'$ mode (b).

and the $A_1'$ mode can be taken as $\omega_A(q) = 405 + 5\sin(qa)$ cm$^{-1}$, where $a = 3.15$ Å is the lattice constant.

Figure S3 shows the size dependence of the Raman shift and linewidth with this model. For the $A_1'$ mode, the Raman frequency blue shifts as the ribbon becomes narrower, while for $E'$ mode, it red shifts. This is due to the different phonon dispersions for the two modes. For the $A_1'$ mode, near $qa \approx 0$, the dispersion $\omega_A(q)$ dictates that phonons with larger momentum have higher frequency, whereas for $E'$ mode, this is opposite. This implies that in nanoribbons where Raman scattering involves phonons with momenta away from the Brillouin zone center, the Raman frequency blue shifts for the $A_1'$ mode but red shifts for the $E'$ mode. Since the amplitude modulation of $\omega_E(q)$ is larger than $\omega_A(q)$, the Raman frequency shift for the $E'$ mode is larger with the same ribbon width. For both modes, the frequency shift and linewidth broadening are very small and may not be observable unless the ribbon is smaller than 5 nm. In Ref. [8], the Raman linewidth broadens and low frequency modes start to appear for ribbons with width of 15 nm. However, for the lithographically patterned nanoribbons here, no clear frequency shift or linewidth broadening is observed with similar ribbon width as shown in Fig. 3, indicating that the helium ion beam milling process could have introduced some structural damage to the monolayer ribbons.

# 4 Multilevel Model of the Nanoribbon PL Emission

In the exciton weak confinement regime, the spatial wavefunction of tightly-bound exciton states is given by the center-of-mass (CM) wavefunction. A simple 1D infinite potential well

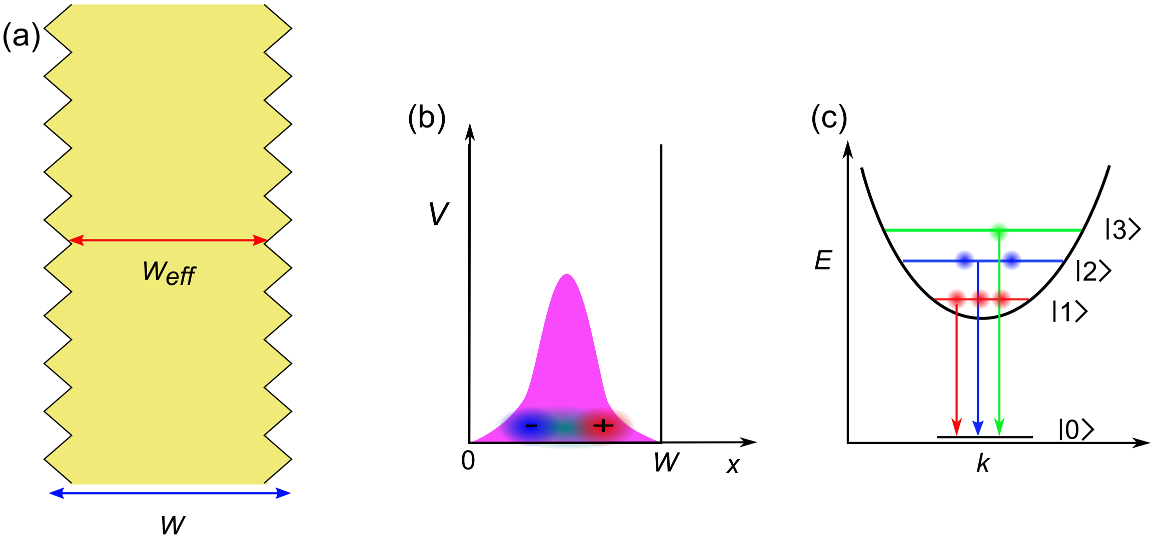


**Figure S4:** Confinement effects in TMD NRs. (a) Lithographically patterned NRs are expected to have edge defects due to the etching process, thus the effective ribbon width is narrower than the physical size. (b) Excitons are confined in the NR structure which can be modelled as an infinite confinement potential well in one dimension. (c) Weak lateral confinement creates closely-spaced energy levels for the center-of-mass motion. With fast recombination from an excited non-equilibrium population, emission from higher spatial energy levels need to be considered.

(Fig. S4(a, b)) leads to a spectrum of energy levels for center-of-mass (CM) states $|n\rangle$ labeled by integer $n$ with the wavefunction and energy as follows:

$$\psi_n(x) = \sqrt{\frac{2}{W}} \sin(k_n x) \tag{S5}$$

$$E_n = \frac{\hbar^2 k_n^2}{2M_{\mathrm{CM}}} \tag{S6}$$

with $k_n = n\pi/W$, $n \in Z : n \geq 0$. This confinement in one-dimension is coupled with a continuous exciton dispersion parallel to the ribbon direction.

Since these levels are generally closely-spaced relative to the homogeneous linewidths (3 meV), the multi-state emission must be considered in a system with short exciton radiative lifetime (Fig. S4(c)) [10]. Excitons radiatively decay before reaching thermal equilibrium through phonon-exciton and exciton-exciton scattering. Here we present a simple toy model that demonstrates how optical pumping of the ensemble of center-of-mass energy levels can lead to an energy shift of the broadened PL spectrum larger than that of a single isolated energy level.

Assuming a non-equilibrium exciton distribution with excitons initially excited uniformly

across the ribbons surface area, the occupation of each spatial wavefunction state can be found by its spatial overlap with the uniform exciton ensemble. The wavefunction of the hot excitons can be expressed as

$$\Phi(x) = \sum_{n=1}^{\infty} C_n \psi_n(x) \tag{S7}$$

with $C_n = \int_0^W \Phi(x)\psi_n(x)^* \mathrm{d}x$. The probability for excitons in the $\psi_n$ state is $|C_n|^2$. Using the wavefunctions in Eq. S5, one can get

$$|C_n|^2 = \frac{8}{(n\pi)^2}, n = 2m + 1 \ (m \in Z : m \geq 0) \tag{S8}$$

Assuming a Gaussian PL emission spectrum from each level of the monolayer $MoS_2$ with exciton center energy of $E_0$ and linewidth parameter $\sigma$, the emission from all states can be weighted and summed. Here, the full-width at half-maximum (FWHM) of the Gaussian spectrum is FWHM $= 2\sqrt{2\ln 2}\sigma$.

$$G_{\mathrm{ML}}(\xi) \propto \exp\left[\frac{-(\xi - E_0)^2}{2\sigma^2}\right] \tag{S9}$$

The emission spectrum of nanoribbons can be written as

$$S_{\mathrm{NR}}(\xi) \propto \sum_{n=1}^{\infty} |C_n|^2 \exp\left[\frac{-(\xi - E_0 - E_n)^2}{2\sigma^2}\right] \tag{S10}$$

The PL energy shift can be extracted by fitting a Gaussian function to $S_{\mathrm{NR}}(x)$ with a typical peak energy $\mathrm{E}_0 = 1.9$ eV and a typical linewidth parameter $\sigma = 0.03$ eV. The variation of the exciton energies and the linewidths in different devices have a minor effect on the extracted shift. This simple toy model neglects the continuous exciton momentum distribution along the ribbons, which can be assumed to lead to quick phonon-mediated relaxation in that direction. This simple model only treats confinement in the weak confinement regime in which distinct energy levels cannot be distinguished and any emission asymmetry is small. Taking into account the first three levels and fitting the experimental data gives parameters of $\delta W = 8$ nm and $M_{\mathrm{CM}} = 0.78m_0$. This result for $M_{\mathrm{CM}}$ from experimental data is close to the value of $\approx 0.9m_0$ in the literature [11, 12]. In contrast, only considering the ground state gives an effective mass $M_{\mathrm{CM}} = 0.21m_0$. Despite the simple assumptions of this toy model and ignoring of microscopic details, it predicts the observed size dependence significantly better than a traditional one state confinement model.

# 5 Electrical transport characterization

Electrical characterization of monolayer $MoS_2$ nanoribbons is carried out by four-terminal transport measurements of field effect transistors. Figure S5(a) shows an optical image of a typical device. The monolayer flake is transferred onto a Si wafer with 285 nm thick thermal oxide, which serves as the back gating dielectric. Nanoribbon arrays are used for this characterization since a single ribbon is vulnerable to damage during processing. In our devices, each array has 70 ribbons patterned. Transport measurements over the temperature range 5 K to 300 K are shown for ribbons with widths of 40 nm and 50 nm.

Figure S5(b-d) show the electrical characterization of the ensemble of NRs. The $I_{\mathrm{sd}}$-$V_{\mathrm{sd}}$ (Fig. S5(b)) curves reveal close to ohmic conduction under low bias, and the conduction is more ohmic at higher temperatures. Figure S5(c) shows the temperature-dependent conductance as a function of back gate voltage. The effective field effect mobility of the NR ensemble is extracted by fitting the $G - V_{\mathrm{g}}$ curve in the linear regime. Figure S5(d) shows the temperature-dependent field effect mobility, where $\mu = \mathrm{d}G/\mathrm{d}V_g \times L/WC_{\mathrm{ox}}$. $L$ and $W$ are the distance of the sensing contacts and the width of ribbons, respectively. $C_{\mathrm{ox}}$ is the capacitance of the gate dielectric. In contrast to the field effect mobility typically measured in a monolayer, where the mobility first increases with temperature and drops down at high temperature before reaching room temperature [13, 14], the effective mobility measured for nanoribbons increases with temperature monotonically, indicating a possible effect from the ribbon edges. The defects along the edges create trap potentials for carriers and the mobility even at room temperature is limited by the local disorder. In contrast, for unpatterned monolayer TMDs, the mobility is limited by phonon scattering at elevated temperatures.

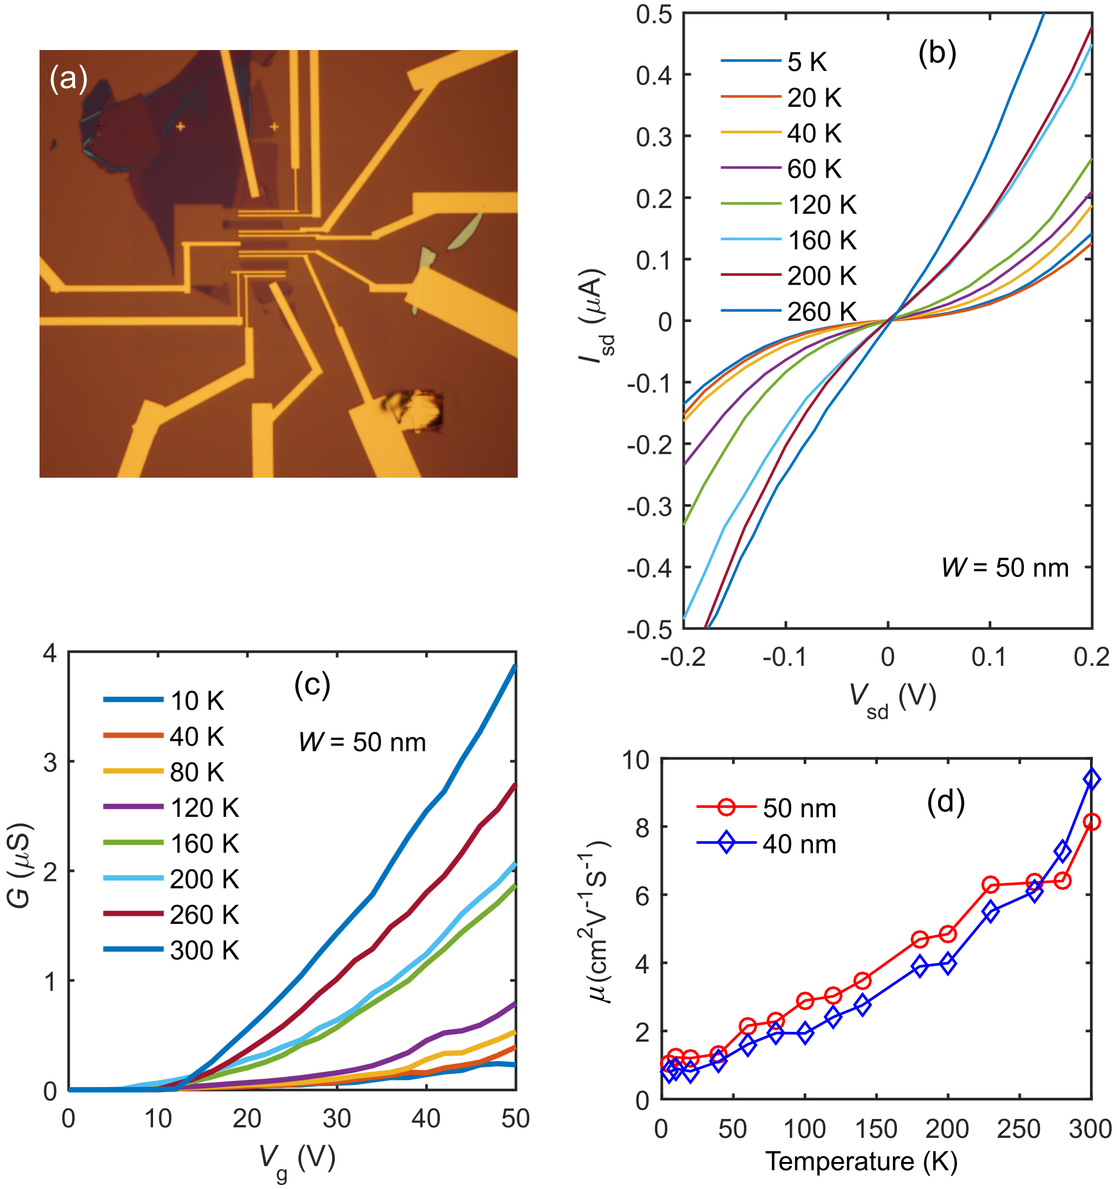


**Figure S5:** Transport characterization of $MoS_2$ nanoribbon array transistors. Each ribbon array has 70 nanoribbons with the same width. (a) $I_{sd}$-$V_{sd}$ for ribbons of 50 nm wide. (b) Gate voltage-dependent of conductance at different temperatures. (c) Field effect mobility extracted by fitting conductance vs. gate voltage in the linear regime. (d) Temperature-dependent field effect mobilities of ribbon arrays with different ribbon width.

# References

[1] Ryu, S., Maultzsch, J., Han, M. Y., Kim, P. & Brus, L. E. Raman spectroscopy of lithographically patterned graphene nanoribbons. *ACS Nano* **5**, 4123–4130 (2011).

[2] Algara-Siller, G., Kurasch, S., Sedighi, M., Lehtinen, O. & Kaiser, U. The pristine atomic structure of $MoS_2$ monolayer protected from electron radiation damage by graphene. *Appl. Phys. Lett.* **103**, 203107 (2013).

[3] Garcia, A. *et al.* Analysis of electron beam damage of exfoliated $MoS_2$ sheets and quantitative HAADF-STEM imaging. *Ultramicroscopy* **146**, 33–38 (2014).

[4] Grigorescu, A. E., van der Krogt, M. C. & Hagen, C. W. Sub-10-nm structures written in ultra-thin HSQ resist layers using electron-beam lithography. In *Advanced Lithography*, 65194A–65194A (International Society for Optics and Photonics, 2007).

[5] Saito, R., Tatsumi, Y., Huang, S., Ling, X. & Dresselhaus, M. Raman spectroscopy of transition metal dichalcogenides. *J. Phys. Condens. Matter* **28**, 353002 (2016).

[6] Zhang, X. *et al.* Phonon and raman scattering of two-dimensional transition metal dichalcogenides from monolayer, multilayer to bulk material. *Chem. Soc. Rev.* **44**, 2757–2785 (2015).

[7] Ferreira, E. M. *et al.* Evolution of the raman spectra from single-, few-, and many-layer graphene with increasing disorder. *Phys. Rev. B* **82**, 125429 (2010).

[8] Wu, J.-B. *et al.* Monolayer molybdenum disulfide nanoribbons with high optical anisotropy. *Adv. Opt. Mater.* **4**, 756–762 (2016).

[9] Molina-Sanchez, A. & Wirtz, L. Phonons in single-layer and few-layer $MoS_2$ and $WS_2$. *Phys. Rev. B* **84**, 155413 (2011).

[10] Moody, G. *et al.* Intrinsic homogeneous linewidth and broadening mechanisms of excitons in monolayer transition metal dichalcogenides. *Nature Commun.* **6**, 8315 (2015).

[11] Cheiwchanchamnangij, T. & Lambrecht, W. R. L. Quasiparticle band structure calculation of monolayer, bilayer, and bulk $MoS_2$. *Phys. Rev. B* **85**, 205302 (2012).

[12] Ramasubramaniam, A. Large excitonic effects in monolayers of molybdenum and tungsten dichalcogenides. *Phys. Rev. B* **86**, 115409 (2012).

[13] Radisavljevic, B. & Kis, A. Mobility engineering and a metal–insulator transition in monolayer $MoS_2$. *Nat. Mater.* **12**, 815–820 (2013).

[14] Xu, S. *et al.* Universal low-temperature Ohmic contacts for quantum transport in transition metal dichalcogenides. *2D Materials* **3**, 021007 (2016).
